# Supplementary material for: Four-Loop Gauge and Three-Loop Yukawa Beta-Functions in a General Renormalizable Theory
Source: arXiv:2105.09918 ancillary file (2021-07-21)
Supplement: Supplementary file 1 [file bCoef.pdf]

# Gauge-coupling beta function coefficients at the four-loop order

|                                                                        |                                                                       |                                                                      |                                                                    |
|------------------------------------------------------------------------|-----------------------------------------------------------------------|----------------------------------------------------------------------|--------------------------------------------------------------------|
| $\mathfrak{g}_1^{(4)} = \frac{160}{9} - \frac{1408}{3}\zeta_3$         | $\mathfrak{g}_2^{(4)} = -\frac{14}{9} + \frac{32}{3}\zeta_3$          | $\mathfrak{g}_3^{(4)} = -\frac{457}{9} + \frac{640}{3}\zeta_3$       | $\mathfrak{g}_4^{(4)} = -\frac{128}{9} + \frac{32}{3}\zeta_3$      |
| $\mathfrak{g}_5^{(4)} = \frac{88}{9} - \frac{64}{3}\zeta_3$            | $\mathfrak{g}_6^{(4)} = -\frac{256}{9} + \frac{832}{3}\zeta_3$        | $\mathfrak{g}_7^{(4)} = -\frac{71}{3} + 8\zeta_3$                    | $\mathfrak{g}_8^{(4)} = -\frac{95}{6} + 16\zeta_3$                 |
| $\mathfrak{g}_9^{(4)} = -\frac{34}{3} + 4\zeta_3$                      | $\mathfrak{g}_{10}^{(4)} = -\frac{23}{3} + 8\zeta_3$                  | $\mathfrak{g}_{11}^{(4)} = \frac{49}{9} - \frac{832}{3}\zeta_3$      | $\mathfrak{g}_{12}^{(4)} = -\frac{3}{2}$                           |
| $\mathfrak{g}_{13}^{(4)} = \frac{92}{27} + \frac{2320}{9}\zeta_3$      | $\mathfrak{g}_{14}^{(4)} = \frac{13733}{108} + \frac{352}{9}\zeta_3$  | $\mathfrak{g}_{15}^{(4)} = \frac{38}{27} + \frac{16}{9}\zeta_3$      | $\mathfrak{g}_{16}^{(4)} = -\frac{181}{27} - \frac{32}{9}\zeta_3$  |
| $\mathfrak{g}_{17}^{(4)} = \frac{28}{27} + \frac{8}{9}\zeta_3$         | $\mathfrak{g}_{18}^{(4)} = -\frac{221}{27} - \frac{16}{9}\zeta_3$     | $\mathfrak{g}_{19}^{(4)} = \frac{158}{9} + \frac{832}{3}\zeta_3$     | $\mathfrak{g}_{20}^{(4)} = \frac{291}{4}$                          |
| $\mathfrak{g}_{21}^{(4)} = -\frac{77}{486}$                            | $\mathfrak{g}_{22}^{(4)} = -\frac{47}{486}$                           | $\mathfrak{g}_{23}^{(4)} = \frac{91}{1944}$                          | $\mathfrak{g}_{24}^{(4)} = \frac{323}{1944}$                       |
| $\mathfrak{g}_{25}^{(4)} = -\frac{769}{486} - \frac{88}{9}\zeta_3$     | $\mathfrak{g}_{26}^{(4)} = -\frac{15025}{1944} - \frac{20}{3}\zeta_3$ | $\mathfrak{g}_{27}^{(4)} = \frac{29}{486}$                           | $\mathfrak{g}_{28}^{(4)} = -\frac{539}{486} - \frac{44}{9}\zeta_3$ |
| $\mathfrak{g}_{29}^{(4)} = \frac{9271}{486} - \frac{448}{9}\zeta_3$    | $\mathfrak{g}_{30}^{(4)} = \frac{60659}{486} - \frac{88}{3}\zeta_3$   | $\mathfrak{g}_{31}^{(4)} = -\frac{12025}{972} - \frac{40}{3}\zeta_3$ | $\mathfrak{g}_{32}^{(4)} = -\frac{49}{486}$                        |
| $\mathfrak{g}_{33}^{(4)} = -\frac{463}{27} - \frac{1676}{9}\zeta_3$    | $\mathfrak{g}_{34}^{(4)} = \frac{5633}{108} + \frac{424}{9}\zeta_3$   | $\mathfrak{g}_{35}^{(4)} = \frac{707}{27} - \frac{1292}{9}\zeta_3$   | $\mathfrak{g}_{36}^{(4)} = \frac{4801}{54} - \frac{176}{9}\zeta_3$ |
| $\mathfrak{g}_{37}^{(4)} = -\frac{85}{27} + \frac{4}{9}\zeta_3$        | $\mathfrak{g}_{38}^{(4)} = -\frac{208}{27} + \frac{16}{9}\zeta_3$     | $\mathfrak{g}_{39}^{(4)} = -\frac{121}{54} + \frac{2}{9}\zeta_3$     | $\mathfrak{g}_{40}^{(4)} = -\frac{641}{108} + \frac{8}{9}\zeta_3$  |
| $\mathfrak{g}_{41}^{(4)} = -\frac{221}{54} + \frac{28}{9}\zeta_3$      | $\mathfrak{g}_{42}^{(4)} = -\frac{1081}{108} + \frac{28}{9}\zeta_3$   | $\mathfrak{g}_{43}^{(4)} = \frac{211}{108} - \frac{22}{9}\zeta_3$    | $\mathfrak{g}_{44}^{(4)} = \frac{53}{216} - \frac{4}{9}\zeta_3$    |
| $\mathfrak{g}_{45}^{(4)} = -\frac{151013}{243} + \frac{440}{9}\zeta_3$ | $\mathfrak{g}_{46}^{(4)} = \frac{37223}{162} + \frac{836}{9}\zeta_3$  | $\mathfrak{g}_{47}^{(4)} = \frac{20873}{432} - \frac{136}{9}\zeta_3$ | $\mathfrak{g}_{48}^{(4)} = -\frac{53}{972}$                        |
| $\mathfrak{g}_{49}^{(4)} = -\frac{4229}{324} - \frac{4}{3}\zeta_3$     | $\mathfrak{g}_{50}^{(4)} = -\frac{59}{1944}$                          | $\mathfrak{g}_{51}^{(4)} = \frac{251}{1296} - \frac{10}{9}\zeta_3$   | $\mathfrak{g}_{52}^{(4)} = -\frac{661}{108} - \frac{26}{9}\zeta_3$ |
| $\mathfrak{g}_{53}^{(4)} = -\frac{7}{216}$                             | $\mathfrak{g}_{54}^{(4)} = -\frac{4}{81}$                             | $\mathfrak{g}_{55}^{(4)} = -\frac{27}{2}$                            | $\mathfrak{g}_{56}^{(4)} = 17$                                     |
| $\mathfrak{g}_{57}^{(4)} = \frac{3}{2}$                                | $\mathfrak{g}_{58}^{(4)} = -\frac{37}{36}$                            | $\mathfrak{g}_{59}^{(4)} = -\frac{5}{36}$                            | $\mathfrak{g}_{60}^{(4)} = \frac{1}{2}$                            |
| $\mathfrak{g}_{61}^{(4)} = \frac{1}{18}$                               | $\mathfrak{g}_{62}^{(4)} = -\frac{5}{3}$                              | $\mathfrak{g}_{63}^{(4)} = -\frac{1}{12}$                            | $\mathfrak{g}_{64}^{(4)} = -\frac{11}{24}$                         |
| $\mathfrak{g}_{65}^{(4)} = -\frac{13}{8}$                              | $\mathfrak{g}_{66}^{(4)} = -\frac{1}{9}$                              | $\mathfrak{g}_{67}^{(4)} = -\frac{1}{12}$                            | $\mathfrak{g}_{68}^{(4)} = \frac{1}{8}$                            |
| $\mathfrak{g}_{69}^{(4)} = -36$                                        | $\mathfrak{g}_{70}^{(4)} = \frac{17}{4}$                              | $\mathfrak{g}_{71}^{(4)} = \frac{3}{2}$                              | $\mathfrak{g}_{72}^{(4)} = 2$                                      |
| $\mathfrak{g}_{73}^{(4)} = \frac{3}{4}$                                | $\mathfrak{g}_{74}^{(4)} = -\frac{59}{24} + 25\zeta_3$                | $\mathfrak{g}_{75}^{(4)} = -\frac{33}{2} - 6\zeta_3$                 | $\mathfrak{g}_{76}^{(4)} = +\frac{49}{4} + 6\zeta_3$               |
| $\mathfrak{g}_{77}^{(4)} = -28 + 15\zeta_3$                            | $\mathfrak{g}_{78}^{(4)} = +\frac{593}{24} + 5\zeta_3$                | $\mathfrak{g}_{79}^{(4)} = 1 - 6\zeta_3$                             | $\mathfrak{g}_{80}^{(4)} = -36\zeta_3$                             |
| $\mathfrak{g}_{81}^{(4)} = -\frac{55}{3} + 10\zeta_3$                  | $\mathfrak{g}_{82}^{(4)} = 29 - 36\zeta_3$                            | $\mathfrak{g}_{83}^{(4)} = -\frac{27}{2}$                            | $\mathfrak{g}_{84}^{(4)} = -\frac{3445}{216} - \frac{7}{9}\zeta_3$ |
| $\mathfrak{g}_{85}^{(4)} = \frac{71}{216} + \frac{8}{9}\zeta_3$        | $\mathfrak{g}_{86}^{(4)} = \frac{359}{432} + \frac{4}{9}\zeta_3$      | $\mathfrak{g}_{87}^{(4)} = -\frac{5093}{216} + \frac{169}{9}\zeta_3$ | $\mathfrak{g}_{88}^{(4)} = -\frac{1259}{36} + 3\zeta_3$            |
| $\mathfrak{g}_{89}^{(4)} = \frac{68}{9} - \frac{22}{3}\zeta_3$         | $\mathfrak{g}_{90}^{(4)} = \frac{463}{216} - \frac{8}{9}\zeta_3$      | $\mathfrak{g}_{91}^{(4)} = \frac{97}{36}$                            | $\mathfrak{g}_{92}^{(4)} = -\frac{4}{9} + \frac{2}{3}\zeta_3$      |
| $\mathfrak{g}_{93}^{(4)} = \frac{679}{432} - \frac{4}{9}\zeta_3$       | $\mathfrak{g}_{94}^{(4)} = \frac{43}{18}$                             | $\mathfrak{g}_{95}^{(4)} = -\frac{1}{18} + \frac{1}{3}\zeta_3$       | $\mathfrak{g}_{96}^{(4)} = -\frac{37}{2}$                          |
| $\mathfrak{g}_{97}^{(4)} = \frac{15}{2}$                               | $\mathfrak{g}_{98}^{(4)} = -\frac{11}{3} + 2\zeta_3$                  | $\mathfrak{g}_{99}^{(4)} = -41$                                      | $\mathfrak{g}_{100}^{(4)} = -\frac{520}{27} + \frac{55}{9}\zeta_3$ |
| $\mathfrak{g}_{101}^{(4)} = \frac{77}{108} - \frac{5}{9}\zeta_3$       | $\mathfrak{g}_{102}^{(4)} = \frac{203}{216} - \frac{5}{18}\zeta_3$    | $\mathfrak{g}_{103}^{(4)} = -\frac{19}{2}$                           | $\mathfrak{g}_{104}^{(4)} = -\frac{823}{18}$                       |
| $\mathfrak{g}_{105}^{(4)} = \frac{109}{36}$                            | $\mathfrak{g}_{106}^{(4)} = \frac{43}{72}$                            | $\mathfrak{g}_{107}^{(4)} = \frac{4721}{216} + \frac{11}{9}\zeta_3$  | $\mathfrak{g}_{108}^{(4)} = -\frac{61}{216} - \frac{1}{9}\zeta_3$  |

|                                                                     |                                                                     |                                                                   |                                                                   |
|---------------------------------------------------------------------|---------------------------------------------------------------------|-------------------------------------------------------------------|-------------------------------------------------------------------|
| $\mathfrak{g}_{109}^{(4)} = -\frac{223}{432} - \frac{1}{18}\zeta_3$ | $\mathfrak{g}_{110}^{(4)} = -4$                                     | $\mathfrak{g}_{111}^{(4)} = -\frac{13}{6}$                        | $\mathfrak{g}_{112}^{(4)} = \frac{1}{4}$                          |
| $\mathfrak{g}_{113}^{(4)} = -\frac{1}{144}$                         | $\mathfrak{g}_{114}^{(4)} = \frac{11}{48}$                          | $\mathfrak{g}_{115}^{(4)} = \frac{20}{3}$                         | $\mathfrak{g}_{116}^{(4)} = 6 - 12\zeta_3$                        |
| $\mathfrak{g}_{117}^{(4)} = +\frac{7}{3} - 24\zeta_3$               | $\mathfrak{g}_{118}^{(4)} = \frac{38}{3}$                           | $\mathfrak{g}_{119}^{(4)} = \frac{2}{3}$                          | $\mathfrak{g}_{120}^{(4)} = -1$                                   |
| $\mathfrak{g}_{121}^{(4)} = -\frac{11}{3}$                          | $\mathfrak{g}_{122}^{(4)} = -\frac{1}{2}$                           | $\mathfrak{g}_{123}^{(4)} = -\frac{19}{6}$                        | $\mathfrak{g}_{124}^{(4)} = -\frac{31}{12} - 6\zeta_3$            |
| $\mathfrak{g}_{125}^{(4)} = \frac{61}{9} - \frac{52}{3}\zeta_3$     | $\mathfrak{g}_{126}^{(4)} = -\frac{9}{2} + 24\zeta_3$               | $\mathfrak{g}_{127}^{(4)} = 2 + 36\zeta_3$                        | $\mathfrak{g}_{128}^{(4)} = \frac{131}{12} - 14\zeta_3$           |
| $\mathfrak{g}_{129}^{(4)} = -\frac{539}{36} - \frac{16}{3}\zeta_3$  | $\mathfrak{g}_{130}^{(4)} = \frac{89}{9} - \frac{38}{3}\zeta_3$     | $\mathfrak{g}_{131}^{(4)} = \frac{87}{8} - 6\zeta_3$              | $\mathfrak{g}_{132}^{(4)} = \frac{43}{12} + 6\zeta_3$             |
| $\mathfrak{g}_{133}^{(4)} = -\frac{1}{2} + \zeta_3$                 | $\mathfrak{g}_{134}^{(4)} = -\frac{301}{72} - \frac{1}{3}\zeta_3$   | $\mathfrak{g}_{135}^{(4)} = -\frac{113}{72} + \frac{1}{3}\zeta_3$ | $\mathfrak{g}_{136}^{(4)} = \frac{80}{9} - \frac{5}{3}\zeta_3$    |
| $\mathfrak{g}_{137}^{(4)} = \frac{11}{6}$                           | $\mathfrak{g}_{138}^{(4)} = \frac{3}{2} + \zeta_3$                  | $\mathfrak{g}_{139}^{(4)} = \frac{1}{6} + \zeta_3$                | $\mathfrak{g}_{140}^{(4)} = -\frac{9}{4} + 3\zeta_3$              |
| $\mathfrak{g}_{141}^{(4)} = \frac{31}{12}$                          | $\mathfrak{g}_{142}^{(4)} = \frac{7}{6}$                            | $\mathfrak{g}_{143}^{(4)} = \frac{23}{3} - 3\zeta_3$              | $\mathfrak{g}_{144}^{(4)} = \frac{113}{144} + \frac{4}{3}\zeta_3$ |
| $\mathfrak{g}_{145}^{(4)} = -\frac{131}{144} - \frac{4}{3}\zeta_3$  | $\mathfrak{g}_{146}^{(4)} = -\frac{779}{144} + \frac{14}{3}\zeta_3$ | $\mathfrak{g}_{147}^{(4)} = \frac{229}{72} - \frac{5}{3}\zeta_3$  | $\mathfrak{g}_{148}^{(4)} = \frac{145}{48} - 3\zeta_3$            |
| $\mathfrak{g}_{149}^{(4)} = \frac{203}{72} + \frac{1}{6}\zeta_3$    | $\mathfrak{g}_{150}^{(4)} = \frac{59}{6}$                           | $\mathfrak{g}_{151}^{(4)} = -\frac{115}{9} + \frac{4}{3}\zeta_3$  | $\mathfrak{g}_{152}^{(4)} = \frac{97}{6}$                         |
| $\mathfrak{g}_{153}^{(4)} = \frac{25}{4}$                           | $\mathfrak{g}_{154}^{(4)} = \frac{10}{9} - \frac{1}{3}\zeta_3$      | $\mathfrak{g}_{155}^{(4)} = \frac{3}{4}$                          | $\mathfrak{g}_{156}^{(4)} = \frac{17}{12}$                        |
| $\mathfrak{g}_{157}^{(4)} = -\frac{373}{144} + \frac{1}{3}\zeta_3$  | $\mathfrak{g}_{158}^{(4)} = 0$                                      | $\mathfrak{g}_{159}^{(4)} = \frac{1}{6}$                          | $\mathfrak{g}_{160}^{(4)} = -\frac{5}{2}$                         |
| $\mathfrak{g}_{161}^{(4)} = -\frac{5}{3}$                           | $\mathfrak{g}_{162}^{(4)} = -\frac{3}{2}$                           | $\mathfrak{g}_{163}^{(4)} = \frac{17}{6} - 3\zeta_3$              | $\mathfrak{g}_{164}^{(4)} = -6$                                   |
| $\mathfrak{g}_{165}^{(4)} = -1$                                     | $\mathfrak{g}_{166}^{(4)} = -1$                                     | $\mathfrak{g}_{167}^{(4)} = -\frac{1}{2}$                         | $\mathfrak{g}_{168}^{(4)} = -\frac{1}{2}$                         |
| $\mathfrak{g}_{169}^{(4)} = -\frac{3}{2}$                           | $\mathfrak{g}_{170}^{(4)} = \frac{34}{9} - \frac{4}{3}\zeta_3$      | $\mathfrak{g}_{171}^{(4)} = -\frac{2}{9} - \frac{4}{3}\zeta_3$    | $\mathfrak{g}_{172}^{(4)} = -\frac{31}{9} + \frac{4}{3}\zeta_3$   |
| $\mathfrak{g}_{173}^{(4)} = -\frac{17}{18} + \frac{4}{3}\zeta_3$    | $\mathfrak{g}_{174}^{(4)} = -\frac{15}{8}$                          | $\mathfrak{g}_{175}^{(4)} = \frac{11}{18} + \frac{2}{3}\zeta_3$   | $\mathfrak{g}_{176}^{(4)} = -\frac{3}{2}$                         |
| $\mathfrak{g}_{177}^{(4)} = -\frac{113}{72} - \frac{1}{6}\zeta_3$   | $\mathfrak{g}_{178}^{(4)} = -\frac{55}{72} - \frac{1}{3}\zeta_3$    | $\mathfrak{g}_{179}^{(4)} = \frac{115}{72} - \frac{1}{6}\zeta_3$  | $\mathfrak{g}_{180}^{(4)} = \frac{9}{8}$                          |
| $\mathfrak{g}_{181}^{(4)} = \frac{11}{18} - \frac{1}{3}\zeta_3$     | $\mathfrak{g}_{182}^{(4)} = \frac{43}{36} - \frac{1}{3}\zeta_3$     | $\mathfrak{g}_{183}^{(4)} = -\frac{115}{72} + \frac{2}{3}\zeta_3$ | $\mathfrak{g}_{184}^{(4)} = -\frac{41}{16}$                       |
| $\mathfrak{g}_{185}^{(4)} = -\frac{3}{8}$                           | $\mathfrak{g}_{186}^{(4)} = -\frac{1}{4}$                           | $\mathfrak{g}_{187}^{(4)} = \frac{19}{96}$                        | $\mathfrak{g}_{188}^{(4)} = -\frac{9}{32}$                        |
| $\mathfrak{g}_{189}^{(4)} = \frac{1}{12}$                           | $\mathfrak{g}_{190}^{(4)} = -\frac{1}{2}$                           | $\mathfrak{g}_{191}^{(4)} = \frac{3}{16}$                         | $\mathfrak{g}_{192}^{(4)} = -\frac{17}{96}$                       |
| $\mathfrak{g}_{193}^{(4)} = -\frac{25}{32}$                         | $\mathfrak{g}_{194}^{(4)} = -\frac{3}{16}$                          | $\mathfrak{g}_{195}^{(4)} = -\frac{1}{4}$                         | $\mathfrak{g}_{196}^{(4)} = \frac{3}{16}$                         |
| $\mathfrak{g}_{197}^{(4)} = \frac{1}{16}$                           | $\mathfrak{g}_{198}^{(4)} = \frac{1}{16}$                           | $\mathfrak{g}_{199}^{(4)} = -4$                                   | $\mathfrak{g}_{200}^{(4)} = -2$                                   |
| $\mathfrak{g}_{201}^{(4)} = \frac{4}{3} - 4\zeta_3$                 | $\mathfrak{g}_{202}^{(4)} = \frac{8}{3} - 8\zeta_3$                 |                                                                   |                                                                   |

# Yukawa-coupling beta function coefficients at the three-loop order

|                                                |                                                |                                                         |                                               |
|------------------------------------------------|------------------------------------------------|---------------------------------------------------------|-----------------------------------------------|
| $\eta_1^{(3)} = -72$                           | $\eta_2^{(3)} = -3$                            | $\eta_3^{(3)} = 33 - 12\zeta_3$                         | $\eta_4^{(3)} = -\frac{3}{2}$                 |
| $\eta_5^{(3)} = \frac{45}{2} - 24\zeta_3$      | $\eta_6^{(3)} = \frac{93}{2}$                  | $\eta_7^{(3)} = -78$                                    | $\eta_8^{(3)} = -12$                          |
| $\eta_9^{(3)} = 102$                           | $\eta_{10}^{(3)} = -48$                        | $\eta_{11}^{(3)} = -9$                                  | $\eta_{12}^{(3)} = -\frac{297}{2}$            |
| $\eta_{13}^{(3)} = \frac{53}{8}$               | $\eta_{14}^{(3)} = \frac{25}{4}$               | $\eta_{15}^{(3)} = 62$                                  | $\eta_{16}^{(3)} = -3$                        |
| $\eta_{17}^{(3)} = 48$                         | $\eta_{18}^{(3)} = -4$                         | $\eta_{19}^{(3)} = -2$                                  | $\eta_{20}^{(3)} = 102$                       |
| $\eta_{21}^{(3)} = -3$                         | $\eta_{22}^{(3)} = -\frac{219}{2}$             | $\eta_{23}^{(3)} = \frac{17}{4}$                        | $\eta_{24}^{(3)} = -4$                        |
| $\eta_{25}^{(3)} = -6$                         | $\eta_{26}^{(3)} = \frac{13}{2}$               | $\eta_{27}^{(3)} = \frac{11}{144}$                      | $\eta_{28}^{(3)} = -\frac{1165}{144}$         |
| $\eta_{29}^{(3)} = \frac{9721}{72}$            | $\eta_{30}^{(3)} = \frac{2}{9}$                | $\eta_{31}^{(3)} = -\frac{925}{72}$                     | $\eta_{32}^{(3)} = \frac{5}{216}$             |
| $\eta_{33}^{(3)} = \frac{181}{27} + 12\zeta_3$ | $\eta_{34}^{(3)} = -\frac{10441}{54}$          | $\eta_{35}^{(3)} = \frac{5}{36}$                        | $\eta_{36}^{(3)} = \frac{19}{27}$             |
| $\eta_{37}^{(3)} = \frac{278}{27} + 24\zeta_3$ | $\eta_{38}^{(3)} = \frac{35}{54}$              | $\eta_{39}^{(3)} = -12$                                 | $\eta_{40}^{(3)} = \frac{5}{4}$               |
| $\eta_{41}^{(3)} = -\frac{17}{48}$             | $\eta_{42}^{(3)} = \frac{19}{16}$              | $\eta_{43}^{(3)} = -\frac{1}{16}$                       | $\eta_{44}^{(3)} = -2 - 144\zeta_3$           |
| $\eta_{45}^{(3)} = 36 - 72\zeta_3$             | $\eta_{46}^{(3)} = 8$                          | $\eta_{47}^{(3)} = \frac{3}{4}$                         | $\eta_{48}^{(3)} = -\frac{23}{4}$             |
| $\eta_{49}^{(3)} = 0$                          | $\eta_{50}^{(3)} = -\frac{9}{4}$               | $\eta_{51}^{(3)} = 44$                                  | $\eta_{52}^{(3)} = -64$                       |
| $\eta_{53}^{(3)} = 6$                          | $\eta_{54}^{(3)} = 22$                         | $\eta_{55}^{(3)} = 0$                                   | $\eta_{56}^{(3)} = 24$                        |
| $\eta_{57}^{(3)} = 16$                         | $\eta_{58}^{(3)} = -4$                         | $\eta_{59}^{(3)} = 64$                                  | $\eta_{60}^{(3)} = -58$                       |
| $\eta_{61}^{(3)} = 4$                          | $\eta_{62}^{(3)} = 10 - 12\zeta_3$             | $\eta_{63}^{(3)} = \frac{65}{4} - 72\zeta_3$            | $\eta_{64}^{(3)} = 80 - 42\zeta_3$            |
| $\eta_{65}^{(3)} = -\frac{59}{2} - 36\zeta_3$  | $\eta_{66}^{(3)} = -15 + 72\zeta_3$            | $\eta_{67}^{(3)} = -\frac{149}{2} + 36\zeta_3$          | $\eta_{68}^{(3)} = 16 + 144\zeta_3$           |
| $\eta_{69}^{(3)} = -\frac{141}{2} + 36\zeta_3$ | $\eta_{70}^{(3)} = -\frac{47}{2} + 72\zeta_3$  | $\eta_{71}^{(3)} = -17$                                 | $\eta_{72}^{(3)} = 15 - 24\zeta_3$            |
| $\eta_{73}^{(3)} = \frac{47}{2} - 36\zeta_3$   | $\eta_{74}^{(3)} = 15 - 48\zeta_3$             | $\eta_{75}^{(3)} = \frac{63}{2} - 36\zeta_3$            | $\eta_{76}^{(3)} = -\frac{11}{2}$             |
| $\eta_{77}^{(3)} = -\frac{11}{8} + 9\zeta_3$   | $\eta_{78}^{(3)} = -\frac{27}{2} + 9\zeta_3$   | $\eta_{79}^{(3)} = \frac{235}{8} - 15\zeta_3$           | $\eta_{80}^{(3)} = -\frac{53}{4} + 36\zeta_3$ |
| $\eta_{81}^{(3)} = 5$                          | $\eta_{82}^{(3)} = -\frac{297}{4} + 36\zeta_3$ | $\eta_{83}^{(3)} = -\frac{83}{4} + 3\zeta_3$            | $\eta_{84}^{(3)} = 17 - 33\zeta_3$            |
| $\eta_{85}^{(3)} = 26 - 6\zeta_3$              | $\eta_{86}^{(3)} = -5$                         | $\eta_{87}^{(3)} = \frac{139}{16} - \frac{3}{2}\zeta_3$ | $\eta_{88}^{(3)} = 5 - 6\zeta_3$              |
| $\eta_{89}^{(3)} = 81$                         | $\eta_{90}^{(3)} = -3$                         | $\eta_{91}^{(3)} = -2$                                  | $\eta_{92}^{(3)} = -19$                       |
| $\eta_{93}^{(3)} = 0$                          | $\eta_{94}^{(3)} = 0$                          | $\eta_{95}^{(3)} = \frac{51}{8}$                        | $\eta_{96}^{(3)} = -\frac{11}{8}$             |
| $\eta_{97}^{(3)} = -\frac{115}{2} + 6\zeta_3$  | $\eta_{98}^{(3)} = 3$                          | $\eta_{99}^{(3)} = 99 - 36\zeta_3$                      | $\eta_{100}^{(3)} = -\frac{5}{4}$             |
| $\eta_{101}^{(3)} = -\frac{25}{4}$             | $\eta_{102}^{(3)} = 2$                         | $\eta_{103}^{(3)} = \frac{61}{2}$                       | $\eta_{104}^{(3)} = -\frac{3}{2}$             |
| $\eta_{105}^{(3)} = -\frac{11}{2}$             | $\eta_{106}^{(3)} = -1$                        | $\eta_{107}^{(3)} = \frac{77}{4} - 9\zeta_3$            | $\eta_{108}^{(3)} = -\frac{11}{8}$            |
| $\eta_{109}^{(3)} = -1$                        | $\eta_{110}^{(3)} = \frac{785}{16} - 3\zeta_3$ | $\eta_{111}^{(3)} = -\frac{43}{16}$                     | $\eta_{112}^{(3)} = -9\zeta_3$                |

|                                                |                                               |                                                          |                                               |
|------------------------------------------------|-----------------------------------------------|----------------------------------------------------------|-----------------------------------------------|
| $\eta_{113}^{(3)} = -\frac{3}{4}$              | $\eta_{114}^{(3)} = -\frac{21}{8}$            | $\eta_{115}^{(3)} = -\frac{9}{4} - 9\zeta_3$             | $\eta_{116}^{(3)} = \frac{1}{8}$              |
| $\eta_{117}^{(3)} = -\frac{3}{4}$              | $\eta_{118}^{(3)} = 0$                        | $\eta_{119}^{(3)} = -\frac{75}{32} + \frac{3}{2}\zeta_3$ | $\eta_{120}^{(3)} = \frac{3}{32}$             |
| $\eta_{121}^{(3)} = \frac{1}{16}$              | $\eta_{122}^{(3)} = 0$                        | $\eta_{123}^{(3)} = -\frac{17}{2}$                       | $\eta_{124}^{(3)} = -17$                      |
| $\eta_{125}^{(3)} = \frac{19}{2}$              | $\eta_{126}^{(3)} = 2$                        | $\eta_{127}^{(3)} = 0$                                   | $\eta_{128}^{(3)} = \frac{3}{2}$              |
| $\eta_{129}^{(3)} = -\frac{3}{8}$              | $\eta_{130}^{(3)} = -\frac{11}{48}$           | $\eta_{131}^{(3)} = 1$                                   | $\eta_{132}^{(3)} = -\frac{5}{32}$            |
| $\eta_{133}^{(3)} = -30$                       | $\eta_{134}^{(3)} = 6$                        | $\eta_{135}^{(3)} = 0$                                   | $\eta_{136}^{(3)} = 10$                       |
| $\eta_{137}^{(3)} = 7$                         | $\eta_{138}^{(3)} = -3$                       | $\eta_{139}^{(3)} = -6$                                  | $\eta_{140}^{(3)} = -26$                      |
| $\eta_{141}^{(3)} = -14$                       | $\eta_{142}^{(3)} = 2$                        | $\eta_{143}^{(3)} = -14$                                 | $\eta_{144}^{(3)} = -12$                      |
| $\eta_{145}^{(3)} = -22$                       | $\eta_{146}^{(3)} = 12$                       | $\eta_{147}^{(3)} = -8$                                  | $\eta_{148}^{(3)} = -6$                       |
| $\eta_{149}^{(3)} = -12$                       | $\eta_{150}^{(3)} = -22$                      | $\eta_{151}^{(3)} = 24$                                  | $\eta_{152}^{(3)} = -22$                      |
| $\eta_{153}^{(3)} = 2$                         | $\eta_{154}^{(3)} = 0$                        | $\eta_{155}^{(3)} = -5$                                  | $\eta_{156}^{(3)} = 3$                        |
| $\eta_{157}^{(3)} = -5$                        | $\eta_{158}^{(3)} = 0$                        | $\eta_{159}^{(3)} = -\frac{3}{2}$                        | $\eta_{160}^{(3)} = \frac{3}{2}$              |
| $\eta_{161}^{(3)} = 0$                         | $\eta_{162}^{(3)} = 0$                        | $\eta_{163}^{(3)} = 3$                                   | $\eta_{164}^{(3)} = -11$                      |
| $\eta_{165}^{(3)} = 0$                         | $\eta_{166}^{(3)} = 0$                        | $\eta_{167}^{(3)} = 0$                                   | $\eta_{168}^{(3)} = -10$                      |
| $\eta_{169}^{(3)} = 34 - 48\zeta_3$            | $\eta_{170}^{(3)} = -8$                       | $\eta_{171}^{(3)} = 4$                                   | $\eta_{172}^{(3)} = \frac{7}{4} - 6\zeta_3$   |
| $\eta_{173}^{(3)} = \frac{7}{4} - 6\zeta_3$    | $\eta_{174}^{(3)} = 2$                        | $\eta_{175}^{(3)} = 36$                                  | $\eta_{176}^{(3)} = -5$                       |
| $\eta_{177}^{(3)} = \frac{11}{2}$              | $\eta_{178}^{(3)} = -11 + 24\zeta_3$          | $\eta_{179}^{(3)} = -17 + 24\zeta_3$                     | $\eta_{180}^{(3)} = -24\zeta_3$               |
| $\eta_{181}^{(3)} = 12 - 12\zeta_3$            | $\eta_{182}^{(3)} = -24 + 24\zeta_3$          | $\eta_{183}^{(3)} = 13 - 12\zeta_3$                      | $\eta_{184}^{(3)} = \frac{35}{8} - 3\zeta_3$  |
| $\eta_{185}^{(3)} = -3 + 9\zeta_3$             | $\eta_{186}^{(3)} = \frac{35}{8} - 3\zeta_3$  | $\eta_{187}^{(3)} = -\frac{13}{8}$                       | $\eta_{188}^{(3)} = -\frac{13}{8}$            |
| $\eta_{189}^{(3)} = -3 + 12\zeta_3$            | $\eta_{190}^{(3)} = -10 + 12\zeta_3$          | $\eta_{191}^{(3)} = -14$                                 | $\eta_{192}^{(3)} = 9\zeta_3 - \frac{31}{4}$  |
| $\eta_{193}^{(3)} = -\frac{51}{4} + 12\zeta_3$ | $\eta_{194}^{(3)} = -8 + 6\zeta_3$            | $\eta_{195}^{(3)} = 1$                                   | $\eta_{196}^{(3)} = -3\zeta_3 - \frac{1}{8}$  |
| $\eta_{197}^{(3)} = 12 + 12\zeta_3$            | $\eta_{198}^{(3)} = \frac{5}{4} + 3\zeta_3$   | $\eta_{199}^{(3)} = -\frac{77}{2} + 12\zeta_3$           | $\eta_{200}^{(3)} = -\frac{47}{8} + 3\zeta_3$ |
| $\eta_{201}^{(3)} = -\frac{67}{8} + 3\zeta_3$  | $\eta_{202}^{(3)} = \frac{87}{4} - 24\zeta_3$ | $\eta_{203}^{(3)} = \frac{13}{2} - 12\zeta_3$            | $\eta_{204}^{(3)} = \frac{25}{4} - 6\zeta_3$  |
| $\eta_{205}^{(3)} = \frac{25}{8} - 6\zeta_3$   | $\eta_{206}^{(3)} = \frac{5}{8} - 3\zeta_3$   | $\eta_{207}^{(3)} = \frac{7}{4} + 12\zeta_3$             | $\eta_{208}^{(3)} = -1 + 3\zeta_3$            |
| $\eta_{209}^{(3)} = -\frac{25}{8} + 3\zeta_3$  | $\eta_{210}^{(3)} = -\frac{11}{2}$            | $\eta_{211}^{(3)} = -\frac{11}{2}$                       | $\eta_{212}^{(3)} = 0$                        |
| $\eta_{213}^{(3)} = -\frac{1}{4} + 3\zeta_3$   | $\eta_{214}^{(3)} = \frac{3}{2} - 12\zeta_3$  | $\eta_{215}^{(3)} = -\frac{29}{8} - 6\zeta_3$            | $\eta_{216}^{(3)} = 5$                        |
| $\eta_{217}^{(3)} = 0$                         | $\eta_{218}^{(3)} = \frac{15}{2} - 6\zeta_3$  | $\eta_{219}^{(3)} = \frac{21}{4} - 3\zeta_3$             | $\eta_{220}^{(3)} = -\frac{9}{2} + 6\zeta_3$  |
| $\eta_{221}^{(3)} = \frac{27}{8} + 3\zeta_3$   | $\eta_{222}^{(3)} = 0$                        | $\eta_{223}^{(3)} = -\frac{3}{4}$                        | $\eta_{224}^{(3)} = 3$                        |
| $\eta_{225}^{(3)} = -2$                        | $\eta_{226}^{(3)} = 4$                        | $\eta_{227}^{(3)} = 5$                                   | $\eta_{228}^{(3)} = 2$                        |
| $\eta_{229}^{(3)} = 6$                         | $\eta_{230}^{(3)} = 2$                        | $\eta_{231}^{(3)} = \frac{5}{8}$                         | $\eta_{232}^{(3)} = \frac{5}{8}$              |

|                                     |                                              |                                     |                                    |
|-------------------------------------|----------------------------------------------|-------------------------------------|------------------------------------|
| $\eta_{233}^{(3)} = 1$              | $\eta_{234}^{(3)} = \frac{3}{2}$             | $\eta_{235}^{(3)} = 1$              | $\eta_{236}^{(3)} = -3$            |
| $\eta_{237}^{(3)} = -4 + 12\zeta_3$ | $\eta_{238}^{(3)} = -6 + 12\zeta_3$          | $\eta_{239}^{(3)} = -8 + 12\zeta_3$ | $\eta_{240}^{(3)} = 2$             |
| $\eta_{241}^{(3)} = 2$              | $\eta_{242}^{(3)} = -4 + 12\zeta_3$          | $\eta_{243}^{(3)} = -6 + 12\zeta_3$ | $\eta_{244}^{(3)} = -5 + 6\zeta_3$ |
| $\eta_{245}^{(3)} = -2 + 3\zeta_3$  | $\eta_{246}^{(3)} = -1 + \frac{3}{2}\zeta_3$ | $\eta_{247}^{(3)} = -3$             | $\eta_{248}^{(3)} = -1$            |
| $\eta_{249}^{(3)} = -1$             | $\eta_{250}^{(3)} = -8$                      | $\eta_{251}^{(3)} = -6$             | $\eta_{252}^{(3)} = 0$             |
| $\eta_{253}^{(3)} = -2$             | $\eta_{254}^{(3)} = -4$                      | $\eta_{255}^{(3)} = 2$              | $\eta_{256}^{(3)} = 4$             |
| $\eta_{257}^{(3)} = \frac{5}{4}$    | $\eta_{258}^{(3)} = -2$                      | $\eta_{259}^{(3)} = 4$              | $\eta_{260}^{(3)} = -2$            |
| $\eta_{261}^{(3)} = -\frac{5}{8}$   | $\eta_{262}^{(3)} = 1$                       | $\eta_{263}^{(3)} = 1$              | $\eta_{264}^{(3)} = 0$             |
| $\eta_{265}^{(3)} = 0$              | $\eta_{266}^{(3)} = -\frac{3}{8}$            | $\eta_{267}^{(3)} = -\frac{3}{4}$   | $\eta_{268}^{(3)} = \frac{7}{4}$   |
| $\eta_{269}^{(3)} = 1$              | $\eta_{270}^{(3)} = \frac{25}{8}$            | $\eta_{271}^{(3)} = \frac{7}{8}$    | $\eta_{272}^{(3)} = -3$            |
| $\eta_{273}^{(3)} = 4$              | $\eta_{274}^{(3)} = 3$                       | $\eta_{275}^{(3)} = -2$             | $\eta_{276}^{(3)} = -3$            |
| $\eta_{277}^{(3)} = \frac{3}{16}$   | $\eta_{278}^{(3)} = \frac{1}{2}$             | $\eta_{279}^{(3)} = 2$              | $\eta_{280}^{(3)} = \frac{1}{8}$   |
| $\eta_{281}^{(3)} = \frac{3}{16}$   | $\eta_{282}^{(3)} = \frac{7}{16}$            | $\eta_{283}^{(3)} = \frac{5}{16}$   | $\eta_{284}^{(3)} = \frac{7}{16}$  |
| $\eta_{285}^{(3)} = 2$              | $\eta_{286}^{(3)} = \frac{25}{8}$            | $\eta_{287}^{(3)} = -3$             | $\eta_{288}^{(3)} = 3$             |
| $\eta_{289}^{(3)} = -1$             | $\eta_{290}^{(3)} = -\frac{3}{16}$           | $\eta_{291}^{(3)} = \frac{9}{16}$   | $\eta_{292}^{(3)} = -\frac{3}{16}$ |
| $\eta_{293}^{(3)} = \frac{9}{16}$   | $\eta_{294}^{(3)} = 1$                       | $\eta_{295}^{(3)} = -\frac{1}{2}$   | $\eta_{296}^{(3)} = -1$            |
| $\eta_{297}^{(3)} = -\frac{5}{16}$  | $\eta_{298}^{(3)} = \frac{1}{32}$            | $\eta_{299}^{(3)} = -\frac{3}{16}$  | $\eta_{300}^{(3)} = -1$            |
| $\eta_{301}^{(3)} = -\frac{1}{4}$   | $\eta_{302}^{(3)} = -\frac{1}{2}$            | $\eta_{303}^{(3)} = -\frac{3}{16}$  | $\eta_{304}^{(3)} = -24$           |
| $\eta_{305}^{(3)} = -12$            | $\eta_{306}^{(3)} = 8 - 24\zeta_3$           | $\eta_{307}^{(3)} = 8 - 24\zeta_3$  | $\eta_{308}^{(3)} = 8 - 24\zeta_3$ |
